# Supplementary material for: Unconventional superconductivity in nearly flat bands in twisted bilayer graphene
Source: arXiv:1803.11190 source file (2019-03-15)
Supplement: Supplementary file 1 [file Supplementary_TBLG.pdf]

# Supplementary Materials: Unconventional superconductivity in nearly flat bands in twisted bilayer graphene

Bitan Roy[1] and Vladimir Juričić[2]

[1]Max-Planck-Institut für Physik komplexer Systeme, Nöthnitzer Stra. 38, 01187 Dresden, Germany

[2]Nordita, KTH Royal Institute of Technology and Stockholm University, Roslagstullsbacken 23, 10691 Stockholm, Sweden

The Supplementary Material contains: (a) Details of the renormalization group (RG) calculation for the Hubbard model at finite temperature ($T$) and finite chemical potential ($\mu$), (b) Details of the mean-field calculation capturing the coexistence of anti-ferromagnetic (AFM) and $E_g$ superconductor, (c) Details of the band diagonalization technique for the $E_g$ pairing in the presence as well as absence of an underlying AFM order.

## I. RG CALCULATION AT FINITE TEMPERATURE AND CHEMICAL DOPING

In the RG calculation presented in the main part of the paper we only considered one of the three quartic terms (the most dominant one) appearing in the Hubbard model, namely $g_2^t$ (see Eq. (3) for definition). For this four-fermion coupling constant we compute the RG flow equation to the one-loop or leading order, yielding

$$\frac{dg_2^t}{d\ell} = -g + 4g^2 \left[ \frac{1}{2} \sum_{\tau=\pm} \tanh\left(\frac{1+\tau\mu}{T}\right) \right], \;\; \frac{dT}{d\ell} = T, \;\; \frac{d\mu}{d\ell} = \mu, \tag{1}$$

along with the flow of temperature and chemical potential. While arriving at the above flow equation we neglected generation of new couplings due to finite $\mu$, which is justified since we are interested in RG flows only to the leading order in $g_2^t$, $\mu$ and $T$. In the above flow equation all parameters are dimensionless defined as $T/(v_F\Lambda) \to T$, $\mu/(v_F\Lambda) \to \mu$ and $g_2^t\Lambda/(\pi v_F) \to g_2^t$. While arriving at the above flow equations we perform summation over fermionic Matsubara frequencies $\omega_n = (2n+1)\pi T$ (setting $k_B = 1$) and integrate out a thin Wilsonian shell $\Lambda e^{-l} < |\mathbf{k}| < \Lambda$. Notice that both temperature and chemical potential are relevant perturbations with scaling dimension $[T] = [\mu] = 1$. Therefore, they respectively introduce infra-red cut-off for the RG flow given by $\ell_*^T = -\log(T(0))$ and $\ell_*^\mu = -\log(\mu(0))$, where the quantity $X(0)$ represents its bare value at $\ell = 0$. Physically these two infra-red cut-off scales correspond to either temperature or chemical potential reaching the ultraviolate energy cut-off $E_\Lambda = v_F\Lambda$, beyond which the notion of Dirac quasiparticles becomes moot. Therefore, we run the coupled RG flow equations for $g_2^t$ only up to a scale $\ell_* = \min.\left(\ell_*^T, \ell_*^\mu\right)$. Now depending on the bare or initial coupling strength $g_2^t(0)$ two situations can arise:

1. $g_2^t(\ell_*) < 1$ which represents a disordered phase of interacting Dirac liquid without any long-range order,
2. $g_2^t(\ell_*) > 1$ which indicates breakdown of the perturbation theory and onset of a broken symmetry phase.

Now to determine the pattern of the symmetry breaking we focus on the RG flow equations for the source terms for anti-ferromagnet ($m$), $E_g$ pairing ($\Delta$) and $A_{1\mathbf{k}}$ pairing ($\Delta'$), which to the leading order are respectively given by

$$\begin{aligned} \frac{d\ln m}{d\ell} - 1 &= \frac{7}{2} g_2^t \left[ \frac{1}{2} \sum_{\tau=\pm} \tanh\left(\frac{1+\tau\mu}{T}\right) \right], \quad \frac{d\ln\Delta}{d\ell} - 1 = \frac{3}{4} g_2^t \left[ \frac{\mu\sinh(1/T) + (1-2\mu^2)\sinh(\mu/T)}{\mu(1-\mu^2)\left[\cosh(1/T) + \cosh(\mu/T)\right]} \right], \\ \frac{d\ln\Delta'}{d\ell} - 1 &= -\frac{3}{4} g_2^t \left[ \frac{2\mu\sinh(\mu/T)}{(1-\mu^2)\left[\cosh(1/T) + \cosh(\mu/T)\right]} \right]. \end{aligned} \tag{2}$$

For brevity we do not display the flow equation for $\Delta'$ in the main text. The quantity appearing on the right hand side of each flow equation corresponds to the scaling dimension of the corresponding order-parameter. Readers can immediately confirm that for any value of $T(<1)$ and $\mu(<1)$ the scaling dimension of $E_g$ pairing is always larger than that for the $A_{1\mathbf{k}}$ pairing. To determine the nature of the broken symmetry phase we simultaneously run the flow of these source terms along with those for $g_2^t$, $T$ and $\mu$ for various choices of their bare values. For the situation (2) (when a broken symmetry phase sets in), the ordered phase represents (1) an AFM if $m(\ell_*) > \Delta(\ell_*)$ or (2) an $E_g$ paired state when $\Delta(\ell_*) > m(\ell_*)$. We subscribe to this procedure to arrive at the phase diagram, shown as Fig. 1 of the main text. Two functions, namely $f(T,\mu)$ and $h(T,\mu)$, introduced in the main text [see Eq. (6)] are

$$f(T,\mu) = \frac{1}{2} \sum_{\tau=\pm} \tanh\left(\frac{1+\tau\mu}{T}\right), \quad h(T,\mu) = \frac{\mu\sinh(1/T) + (1-2\mu^2)\sinh(\mu/T)}{\mu(1-\mu^2)\left[\cosh(1/T) + \cosh(\mu/T)\right]}. \tag{3}$$

## II. MEAN-FIELD ANALYSIS FOR COMPETING ANTIFERROMAGNET AND SUPERCONDUCTOR

The RG technique we highlighted in the previous section can only be used to determine the phase boundary between an interacting but disordered Dirac liquid and AFM or superconducting order in an unbiased fashion. However, inside any ordered phase the above RG breaks down as the four-fermion coupling constant, namely $g^t_2$, *diverges* (thus indicating onset of a broken symmetry phase). Inside the ordered phase there exists yet another interesting scenario: *a possible coexistence of AFM and superconducting orders.* In order to capture such coexistence, we therefore have to rely on a mean-field analysis with these two competing orders. The mean-field free energy at finite temperature in the presence of these two orderings takes the form

$$F\left(m,\Delta,\mu\right)=\frac{m^2}{2g_1}+\frac{|\Delta|^2}{4g_2}-2\sum_{j=1,2}\int' \frac{d^2\mathbf{k}}{(2\pi)^2}E_j\left(\mathbf{k},m,\Delta,\mu\right)-4T\sum_{j=1,2}\int' \frac{d^2\mathbf{k}}{(2\pi)^2}\log\left[1+\exp\left(-\frac{E_j\left(\mathbf{k},m,\Delta,\mu\right)}{T}\right)\right], \quad (4)$$

where $g_1$ and $g_2$ are two effective (phenomenological) interactions, respectively conducive for AFM and superconducting orders and

$$E_j\left(\mathbf{k},m,\Delta,\mu\right)=\left[v^2k^2+\mu^2+m^2+|\Delta|^2+(-1)^j\sqrt{2k^2|\Delta|^2(1-\sin 2\theta_{\mathbf{k}})+4(k^2+m^2)\mu^2}\right]^{1/2}. \quad (5)$$

Here $\theta_{\mathbf{k}}$ is the polar angle in the momentum space. The integral over momentum is restricted up to an ultraviolet momentum cut-off $\Lambda$. To proceed with the analysis, we first introduce a set of dimensionless variables according to

$$\frac{k}{\Lambda}\to k,\ \frac{m}{v_F\Lambda}\to m,\ \frac{\Delta}{v_F\Lambda}\to\Delta,\ \frac{\mu}{v_F\Lambda}\to\mu,\ \frac{T}{v_F\Lambda}\to T,\ \frac{2g_j\Lambda}{v_F}\to g_j,\ \frac{E_j}{v_F\Lambda}\to E_j,\ f=F\Lambda^2/(v_F\Lambda), \quad (6)$$

where $j=1,2$ and $f$ is the dimensionless free-energy density.

Finally, we minimize the dimensionless free-energy density with respect to two order-parameters ($m$ and $\Delta$) to arrive at the following coupled self-consistent gap equations

$$\frac{1}{g_1} = 2\int_0^{2\pi}\int_0^1 \frac{kdkd\theta_{\mathbf{k}}}{(2\pi)^2}\sum_{j=1,2}\frac{\partial E_j}{\partial m^2}-4\sum_{j=1,2}\int_0^{2\pi}\int_0^1\frac{kdkd\theta_{\mathbf{k}}}{(2\pi)^2}\frac{\exp[-E_j/T]}{1+\exp[-E_j/T]}\frac{\partial E_j}{\partial m^2}, \quad (7)$$

$$\frac{1}{g_2} = 4\int_0^{2\pi}\int_0^1 \frac{kdkd\theta_{\mathbf{k}}}{(2\pi)^2}\sum_{j=1,2}\frac{\partial E_j}{\partial \Delta^2}-4\sum_{j=1,2}\int_0^{2\pi}\int_0^1\frac{kdkd\theta_{\mathbf{k}}}{(2\pi)^2}\frac{\exp[-E_j/T]}{1+\exp[-E_j/T]}\frac{\partial E_j}{\partial \Delta^2}. \quad (8)$$

In the last set of equations we have dropped the explicit dependence of $E_j$s on its arguments for brevity. This set of gap equations captures nontrivial solutions for two order-parameters $m$ and $\Delta$, besides the trivial ones, i.e. $m=0$ and/or $\Delta=0$. We numerically solve these two coupled gap equations for a specific fixed values of $g_1$ and $g_2$ to arrive at the phase diagram, shown as Fig. 2 in the main text. This phase diagram besides pure AFM and superconducting phases, also displays a regime where these two phases can coexist.

## III. BAND DIAGONALIZATION PROCEDURE FOR THE PAIRINGS

We here present the procedure for obtaining the form of a pairing near the Fermi surface in the conduction band of the parent Dirac Hamiltonian, which describes the low-energy excitations near the charge-neutrality point and possibly around the nearly flat electronic bands close to 1/4 and 3/4 fillings (see main text for discussion on this issue), in the twisted bilayer graphene close to the magic angle (MA-TBLG) as given by Eq. (1) in the main text. We first diagonalize the $2\times 2$ Dirac Hamiltonian of the form

$$H(\mathbf{k},v,m,\mu)=v\left(\sigma_1k_1-\sigma_2k_2\right)+m\,\sigma_3-\mu\,\sigma_0, \quad (9)$$

with $\mu>0$. The spectrum of the Hamiltonian is $E_\pm(k,v,m,\mu)=\pm\sqrt{v^2k^2+m^2}-\mu$, with $\pm$ corresponding to the conduction and the valence band. The corresponding wave-functions can be compactly written as

$$|\pm,\mathbf{k},v,m\rangle=A_\pm(k,v,m)\begin{pmatrix}\pm e^{i\phi}\left(\sqrt{k^2v^2+m^2}\pm m\right)\\ kv\end{pmatrix}, \quad (10)$$

with the normalization factor

$$A_{\pm}(k,v,m) = \frac{1}{\left[2\sqrt{k^2v^2+m^2}\left(\sqrt{k^2v^2+m^2}\pm m\right)\right]^{1/2}}. \tag{11}$$

Here, $(k,\phi)$ are the polar coordinates in the momentum space, $k_1 = k\cos\phi, k_2 = k\sin\phi$, and $\boldsymbol{\sigma}$ are the two-dimensional Pauli matrices. The matrix diagonalizing the above 'master' Hamiltonian in terms of the bands reads

$$U(\mathbf{k},v,m) = (|+,\mathbf{k},v,m\rangle, |-,\mathbf{k},v,m\rangle)^\top, \tag{12}$$

and in the band representation

$$\mathrm{diag}(E_+(k,v,m,\mu), E_-(k,v,m,\mu)) = U^\dagger(\mathbf{k},v,m)\, H(\mathbf{k},v,m,\mu)\, U(\mathbf{k},v,m). \tag{13}$$

The Hamiltonian in Eq. (1) of the main text in the presence of AFM order, oriented in the $z$ direction, reads as

$$H_{D,AF}(\mathbf{k},v,m,\mu) = v\sigma_0(\alpha_3\beta_1 k_1 - \alpha_0\beta_2 k_2) + m\sigma_3\alpha_0\beta_3, \tag{14}$$

with $\boldsymbol{\sigma},\boldsymbol{\alpha},\boldsymbol{\beta}$ as three sets of Pauli matrices respectively acting on the spin, valley and the sublattice space, and $v \equiv v_F$ (for notational consistency with the main text). The above Hamiltonian can be rewritten in terms of the 'master' Hamiltonian in Eq. (9) according to

$$H_{D,AF}(\mathbf{k},m) = H(k_1,k_2,m) \oplus H(-k_1,k_2,m) \oplus H(k_1,k_2,-m) \oplus H(-k_1,k_2,-m)], \tag{15}$$

and for clarity we have omitted the arguments $v$ and $\mu$, which are implicitly assumed. Therefore, the corresponding diagonalizer in the band basis reads

$$\begin{aligned} U^\top = \mathrm{diag}[&|+,k,\phi,m\rangle, |+,k,\pi-\phi,m\rangle, |+,k,\phi,-m\rangle, |+,k,\pi-\phi,-m\rangle, \\ &|-,k,\phi,m\rangle, |-,k,\pi-\phi,m\rangle, |-,k,\phi,-m\rangle, |-,k,\pi-\phi,-m\rangle]. \end{aligned} \tag{16}$$

In the Nambu doubled basis the effective single-particle Hamiltonian takes the form

$$H_0 = \eta_3\sigma_0\alpha_0\left[\sqrt{v^2k^2+m^2} - \mu\right], \tag{17}$$

where the newly introduced Pauli matrices $\boldsymbol{\eta}$ operate on particle-hole or Nambu index. In the presence of an AFM order we can perform a *large mass expansion*, leading $H_0 \to \eta_3\left[k^2/(2m) - \mu_*\right]$, while in the absence of AFM order (setting $m=0$) we find $H_0 \to \eta_3\left[vk - \mu\right]$, as announced in the main text. Here, $\mu_* = \mu - m$ is the effective chemical potential, measured from the bottom of the conduction band.

Now, taking the form of the two-component $E_g$ pairing $\Delta_{E_g} = \Delta\sigma_0(\Gamma_1,\Gamma_2) \equiv \Delta\sigma_0(\alpha_3\beta_2, \alpha_0\beta_1)$, and projecting its components onto the conduction and valence bands using the above matrix, we obtain the form of the pairing in the conduction band

$$U^\dagger\sigma_0\Gamma_1 U \to\sim \sigma_0\alpha_3\frac{k_y}{\sqrt{v^2k^2+m^2}}, \quad U^\dagger\sigma_0\Gamma_2 U \to\sim \sigma_0\alpha_3\frac{k_x}{\sqrt{v^2k^2+m^2}}, \tag{18}$$

Assuming that the pairing interaction exists only around the Fermi surface, we can now replace $\sqrt{v^2k^2+m^2}$ by $k_F$ the Fermi momentum. Specifically, in the presence or absence of the AFM order we respectively find $k_F \approx \sqrt{2m\mu/v_F}$ and $k_F = \sqrt{\mu/v_F}$. Therefore, the $E_g$ pairing represents a $p$-wave valley triplet and spin singlet, as stated in the main text. We stress that the emergent $p$-wave nature of the $E_g$ pairing in the proximity to the Fermi surface solely stems from the fact that the normal state band structure is described by either massive (in the presence of AFM order) or massless (in the absence of AFM order) Dirac fermions. The same band-diagonalization procedure can be adopted to find the form of pairings close to 1/4 and 3/4 fillings, where bands are *nearly* flat, but can possibly be described in terms of slow Dirac fermions. The only difference is that now the chemical potential $\mu$ is now measured from the center of the nearly flat bands, placed at 1/4 and 3/4 fillings.
